# Supplementary material for: Two New Upper Bounds for the Maximum k-plex Problem
Source: arXiv:2301.07300 source file (2024-01-19)
Supplement: Supplementary file 1 [file Appendix.tex]

A k-plex in a graph is a vertex set where each vertex is non-adjacent to at most k vertices (including itself) in this set, and the Maximum k-plex Problem (MKP) is to find the largest k-plex in the graph. As a practical NP-hard problem, MKP has many important real-world applications, such as the analysis of various complex networks. Branch-and-bound (BnB) algorithms are a type of well-studied and effective exact algorithms for MKP. Recent BnB MKP algorithms involve two kinds of upper bounds based on graph coloring and partition, respectively, that work in different perspectives and thus are complementary with each other. In this paper, we first propose a new coloring-based upper bound, termed Relaxed Graph Color Bound (RelaxGCB), that significantly improves the previous coloring-based upper bound. We further propose another new upper bound, termed RelaxPUB, that incorporates RelaxGCB and a partition-based upper bound in a novel way, making use of their complementarity. We apply RelaxGCB and RelaxPUB to state-of-the-art BnB MKP algorithms and produce eight new algorithms. Extensive experiments using diverse k values on hundreds of instances based on dense and massive sparse graphs demonstrate the excellent performance and robustness of our proposed methods.

\newpage
\twocolumn[
\begin{@twocolumnfalse}
\section*{\centering{\LARGE{Appendix of ``New Upper Bounds for the Maximum k-plex Problem''}}}
~\\
\end{@twocolumnfalse}
]

In the Appendix, we mainly present some supplementary experiments. We first present comparison results between the baseline algorithms and our produced new algorithms on the 10th DIMACS benchmark that contains 82 graphs with up to 2 \times 10^7 vertices. For each 10th DIMACS graph, we also generate six MKP instances with k \in [2,7], and set the cut-off time to 1,800 seconds.

Then, we present some representative MKP instances to see how many times our proposed SeesawUB selects the extractions obtained by each of BarrelUB and DisePUB, i.e., how many times they win the seesaw playing game, respectively, so as to further show their complementarity and performance on different instances.

\section{Comparison on the 10th DIMACS benchmark}
Results of the number of 10th DIMACS instances with different k values that can be solved by each algorithm within 1,800 seconds are summarized in Table~\ref{table-Appendix}. 

\begin{table}[h]
\centering
\footnotesize
\begin{tabular}{l|rrrrrr} \bottomrule
\diagbox{Algorithm}{$k$}             & 2  & 3  & 4  & 5  & 6  & 7  \\ \hline
Barrel-Maplex & 62 & \textbf{47} & 41 & 32 & \textbf{37} & \textbf{30} \\
Maplex        & 62 & 46 & 41 & 32 & 36 & 29 \\ \hline
Seesaw-kPlexS & 67 & 67 & 67 & 67 & 67 & 67 \\
kPlexS        & 67 & 67 & 67 & 67 & 67 & 67 \\ \hline
SeesawMKP     & 63 & 61 & 52 & 50 & 52 & \textbf{50} \\
DiseMKP       & 63 & 61 & 52 & \textbf{51} & \textbf{54} & 46 \\ \hline
Seesaw-KPLEX  & 76 & 76 & 76 & 76 & 76 & 75 \\
KPLEX         & 76 & 76 & 76 & 76 & 76 & 75   \\ \toprule
\end{tabular}
\caption{Comparison on the 10th DIMACS benchmark. Unique better results are appeared in bold.}
\label{table-Appendix}
\end{table}

From the results, we can observe that each baseline and the corresponding new algorithm with our proposed upper bounds show similar performance on 10th DIMACS instances. This is because most of the 10th DIMACS graphs are either too hard or too easy for each baseline algorithm. For example, there is only one among all the 492 instances that can be solved by KPLEX within more than 100 and less than 1,800 seconds, and only 16 among all the 492 instances that can be solved by KPLEX within more than 10 and less than 1,800 seconds.

\section{Records of the Seesaw Playing Game}
