# Supplementary material for: Two New Upper Bounds for the Maximum k-plex Problem
Source: arXiv:2301.07300 source file (2024-01-19)
Supplement: Supplementary file 2 [file table-Appendix.tex]

\begin{table}[h]
\centering
\footnotesize
\begin{tabular}{l|rrrrrr} \bottomrule
\diagbox{Algorithm}{$k$}             & 2  & 3  & 4  & 5  & 6  & 7  \\ \hline
Barrel-Maplex & 62 & \textbf{47} & 41 & 32 & \textbf{37} & \textbf{30} \\
Maplex        & 62 & 46 & 41 & 32 & 36 & 29 \\ \hline
Seesaw-kPlexS & 67 & 67 & 67 & 67 & 67 & 67 \\
kPlexS        & 67 & 67 & 67 & 67 & 67 & 67 \\ \hline
SeesawMKP     & 63 & 61 & 52 & 50 & 52 & \textbf{50} \\
DiseMKP       & 63 & 61 & 52 & \textbf{51} & \textbf{54} & 46 \\ \hline
Seesaw-KPLEX  & 76 & 76 & 76 & 76 & 76 & 75 \\
KPLEX         & 76 & 76 & 76 & 76 & 76 & 75   \\ \toprule
\end{tabular}
\caption{Comparison on the 10th DIMACS benchmark. Unique better results are appeared in bold.}
\label{table-Appendix}
\end{table}
